# Supplementary material for: Active Learning for Control-Oriented Identification of Nonlinear Systems
Source: arXiv:2404.09030 source file (2024-08-13)
Supplement: Supplementary file 1 [file appendix_doed.tex]

\section{Modifications to Dynamic Optimal Experiment Design}

\subsection{Dynamic Optimal Experiment Design}
\label{s: doed}

We consider an experiment design procedure, \Cref{alg: doed}, which is a modified version of the algorithm from \citet{wagenmaker2023optimal}. The goal of this algorithm is to collect a dataset consisting of $N$ episodes playing exploration policies belonging to $\Pi_{\exp}$ whose Gram matrix $\Lambda$ \eqref{eq: Gram matrices} which approximately minimizes the objective $\Phi(\Lambda)$. It takes as input the objective $\Phi$, an episode budget $N$, an initial exploration policy $\pi^0$, a parameter estimate $\hat\phi$, and a confidence set for the parameters $\calB$. The  algorithm plays a sequence of $N^{1/3}$ epochs, each with $N^{2/3}$ episodes. For the first epoch, it plays the initial policy to set an initial value of the Gram matrix $\Lambda_0$. Starting from this value, the algorithm performs a variant of gradient descent on the objective $\Phi$, where each epoch is a gradient step. At each iteration, it computes the gradient $\Xi_n$ of this objective at the current iterate $\Lambda_n$. Rather than taking a step in the direction $\Xi_n$, it takes a step in the descent direction constrained to the set of Gram matrices achievable under the dynamics evolve according to \eqref{eq: dyn} when the input is chosen according to some  exploration policy $\pi \in \Pi_{\exp}$. It does so by estimating the solution to 
\begin{align*}
    \underset{\tilde \pi \in \Pi_{\exp}}{\min}  \E_{\pi, \phi^\star}\brac{\sum_{t=1}^{T} c^n(X_t,U_t)}, 
\end{align*}
where $c^n$ is defined in terms of the gradient $\Xi_n$ as 
\begin{align*}
    c^n(x,u) = \frac{ \trace\paren{Df(x,u;\hat\phi)  \Xi_n Df(x,u;\hat\phi)^\top}}{B_{\Phi}}.
\end{align*}
In the above optimization problem, the expectation is taken with respect to the true parameter, which is unknown. 
However, the confidence ball $\calB$ centered at the estimate $\hat \phi$ can be used to approximate the solution. In particular, the algorithm applies optimism in the face of uncertainty \citep{abbasi2011improved, kakade2020information} to select the exploration policy which solves the problem
\begin{align*}
    \underset{\tilde \pi \in \Pi_{\exp}}{\min}  \min_{\phi \in \calB} \E_{\pi, \phi}\brac{\sum_{t=1}^{T} c^n(X_t,U_t)}. 
\end{align*}
Doing so allows us to achieve high probability bounds on the objective value obtained by the dynamic optimal experiment design algorithm \eqref{eq: doed success}. The formal version of this is modified from Theorem 3 of \citet{wagenmaker2023optimal}, and is presented in \Cref{thm: doed closeness}. 

\begin{algorithm}
\caption{$\texttt{DOED+}(\Phi, N, \pi^0, \hat \phi, \calB,  B_{\Phi})$} 
\label{alg: doed}
\begin{algorithmic}[1]
\State \textbf{Input:} Objective $\Phi$, episodes $N$, initial exploration policy $\pi^0$, parameter estimate $\hat \phi$, parameter uncertainty set $\calB$, smoothness bound $B_{\Phi}$ 
% \State Choose $B_{\Phi}$ satisfying the boundedness condition of Assumption~\ref{asmp: doed regularity}
\State Set $\tilde N \gets \lfloor N^{2/3} \rfloor$, $\tilde K \gets \lfloor N^{1/3} \rfloor - 1$, $\gamma_n \gets \frac{1}{n+1}$.
\State Play $\pi^0$ for $\tilde N$ episodes to collect $\curly{X_t^n, U_t^n}_{t, n=1}^{T+1,\tilde N}$,
\State Store $\calD_0 \gets \curly{X_t^n, U_t^n}_{t, k=1}^{T+1,\tilde N}$
\State Form the Gram matrix $\Delta_0 = \frac{1}{\tilde N}\sum_{{t, n=1}}^{T,\tilde N} D f(X_t^n, U_t^n; \hat \phi)^\top D f(X_t^n, U_t^n; \hat \phi)$
\For{$k=1,\dots, \tilde K$}
\State Define $\Xi_k \gets \nabla_{\Lambda} \Phi(\Lambda)\vert_{\Lambda = \Lambda_{k-1}}$ and $c^k(x,u) \!\gets\! \frac{ \trace\paren{Df(x,u;\hat\phi)  \Xi_k Df(x,u;\hat\phi)^\top}}{B_{\Phi}}$
\State \label{line: optimistic synth}Set $\pi^k \gets \underset{\tilde \pi \in \Pi_{\exp}}{\argmin} \,\underset{\phi \in \calB}{\min} \E_{\pi, \phi}\brac{\sum_{t=1}^{T} c^k(X_t,U_t)}$
\State Run $\pi^k$ for $\tilde N$ episodes, collecting $\curly{X_t^n, U_t^n}_{t, n=1}^{T,\tilde N}$, and update the dataset and Gram matrix as 
\begin{align*}\Lambda_k &\gets (1-\gamma_k) \Lambda_{k-1} + \frac{\gamma_k}{\tilde N} \sum_{t,n=1}^{T,\tilde N} Df(x,u;\hat\phi)^\top \paren{\Xi_k} Df(x,u;\hat\phi), \quad \calD_{k} \gets \calD_{k-1} \cup \curly{X_t^n, U_t^n}_{t, n=1}^{T+1,\tilde N}
\end{align*}
\EndFor
\State \textbf{Return: $\Lambda_{\tilde K}$, $\curly{\pi^k}_{k=1}^{\tilde K}$}
\end{algorithmic}
\end{algorithm}

\subsection{Proof of correctness for $\texttt{DOED}_+$ Algorithm}

The objective of \Cref{alg: doed} is to collect data $\curly{X_t^n, U_t^n}_{n,t=1}^{N,T}$ from the system to optimize the some objective $\Phi(\Lambda)$, where 
\begin{align*}
    \Lambda = \sum_{n,t=1}^{N,T} Df(X_t^n, U_t^n; \hat\phi)^\top Df(X_t^n, U_t^n; \hat\phi).
\end{align*}
In light of this, we define the set of all possible Gram  matrices corresponding to the parameter parameter $\hat\phi$:
\begin{align*}
    \Omega(\phi) &= \bigg\{\sum_{t=1}^T D f(x_t, u_t;\phi)^\top D f(x_t, u_t;\phi): x_t \in \R^{\dx}, u_t \in \R^{\du}, \forall h\in[H]\bigg\}.
\end{align*}

The correctness of the algorithm can be guaranteed under the following regularity assumption on the objective.
\begin{assumption}
    \label{asmp: doed regularity}
    The objective $\Phi$ is convex and differentiable. Additionally, it is $\kappa$ smooth in that for the dual norm $\norm{\cdot}_{\star}$ of $\norm{\cdot}$, 
    \begin{align*}
        \norm{ \nabla \Phi(\Lambda) - \nabla \Phi(\Lambda')}_{\star} \leq \kappa \norm{\Lambda - \Lambda'} \,\,\,\,\forall \Lambda, \Lambda' \in \Omega(\hat \phi). 
    \end{align*}
    Furthermore, suppose there exists some $B_{\Phi} <\infty$ such that for all $\Lambda \in \Omega(\hat \phi), x\in\R^{\dx}, u \in \R^{\du}$,
    \begin{align*}
         \norm{D f(x,u,\hat\phi) \nabla \Phi(\Lambda)D f(x,u,\hat\phi)^\top } \leq B_{\Phi}. 
    \end{align*}
\end{assumption}

This leads us to the following result, characterizing the optimality of the data collected via the dynamic optimal experiment design procedure. 
\begin{theorem}[Modification of Theorem 3 of \citet{wagenmaker2023optimal}]
    \label{thm: doed closeness}
    Suppose Assumptions~\ref{asmp: smooth dynamics} and \ref{asmp: doed regularity} hold. 
    Additionally, suppose that $\phi^\star \in \calB$. Let $D(\calB) = \sup_{\phi_1, \phi_2 \in \calB^-} \norm{\phi_1 - \phi_2}$. Then with probability at least $1-\delta$, the data collected at the final round of $\texttt{DOED}_+$ satisfies
    \begin{align*}
        &\Phi\paren{\frac{1}{(\tilde K+1) \tilde N} \sum_{t,n=1}^{T((\tilde K+1) \times \tilde N)} D f(X_t^n, U_t^n; \hat \phi)^\top D f(X_t^n, U_t^n; \hat \phi) }- \min_{\pi \in \Pi_{\exp}} \Phi\paren{\E_{\pi, \phi^\star}\brac{ \sum_{t=1}^{T} D f(X_t^1, U_t^1; \hat \phi)^\top D f(X_t^1, U_t^1; \hat \phi)}} \\
        &\leq \frac{2 \kappa T^2 L_f^4 \log(\tilde K+1)}{\tilde K+1} \!+\!B_{\Phi} \paren{\frac{T^2 L_f D(\calB)}{\sigma_w} \! +\! \sqrt{\frac{8 \log\frac{2\tilde K}{\delta}}{\tilde N}}}.   
    \end{align*}
\end{theorem}
To prove the above result, we first present an extension of the simulation lemma from \citet{kakade2020information} to the setting of smooth nonlinear systems. 

\begin{lemma}[Self-Bounding, Simulation Lemma: Modified from \citet{kakade2020information}] 
    \label{lem: self-bounding}
    Suppose Assumption~\ref{asmp: smooth dynamics} holds. For any policy $\pi$, model parameters $\phi$ and non-negative cost $c$ satisfying $c < 1$, it holds that
    \begin{align*}
        \E_{\pi, \phi^\star}\brac{\sum_{t=1}^T c (X_t,U_t)} -  \E_{\pi, \phi}\brac{\sum_{t=1}^T c (X_t,U_t)} \leq \frac{T^2 L_f}{\sigma_w} \norm{\phi - \phi^\star}. 
    \end{align*}
\end{lemma}
\begin{proof}
    The proof follows as in the proof of Lemma B.3 of \citet{kakade2020information}. 
    Consider a state/input pair $(X_t, U_t)$ from rolling out the policy $\pi$ on the system $\phi^\star$. Where \citet{kakade2020information} apply the bound on the difference in means between two Gaussian distributions, we use the Gaussian distributions describing the next state update from $X_t, U_t$ under the model described by $\phi$ and by $\phi^\star$: $\calN(f(X_t, U_t; \phi^\star), \sigma_w^2)$ and $\calN(f(X_t, U_t; \phi), \sigma_w^2)$. This results in a bound on the quantity of interest as
    \begin{align*}
        &\E_{\pi, \phi^\star}\brac{\sum_{t=1}^T c (X_t,U_t)} -  \E_{\pi, \phi}\brac{\sum_{t=1}^T c (X_t,U_t)} \\
        &\leq \sqrt{T \E_{\pi, \phi^\star}\brac{\paren{\sum_{t=1}^T c(X_t, U_t)}^2 }} \sqrt{\E_{\pi, \phi^\star} \brac{\sum_{t=1}^T \min\curly{\frac{1}{\sigma_w^2} \norm{f(X_t, U_t, \phi^\star) - f(X_t, U_t, \phi)}^2 , 1}} }. 
    \end{align*}
    Using the fact that the cost is bounded by one, we have 
    \begin{align*}
        \E_{\pi, \phi^\star}\brac{\paren{\sum_{t=1}^T c(X_t, U_t)}^2 } \leq T^2 
    \end{align*}
    For the remaining quantity, we may  bound 
    \begin{align*}
         \E_{\pi, \phi^\star} \brac{\sum_{t=1}^T \min\curly{\frac{1}{\sigma_w^2} \norm{f(X_t, U_t, \phi^\star) - f(X_t, U_t, \phi} , 1}}  &\leq \frac{1}{\sigma_w^2} \E_{\pi, \phi^\star} \brac{\sum_{t=1}^T  \norm{f(X_t, U_t, \phi^\star) - f(X_t, U_t, \phi)}^2} \\
         &= \frac{1}{\sigma_w^2} \E_{\pi, \phi^\star} \brac{\sum_{t=1}^T  \norm{Df(X_t, U_t, \tilde \phi)(\phi^\star - \phi)}^2} \\ 
         &\leq \frac{TL_f^2}{\sigma_w^2} \norm{\phi^\star -\phi}^2. 
    \end{align*}
    The equality follows by a first order Taylor expansion of $f$ about $\phi^\star$. Here $\tilde \phi$ is a convex combination of $\phi$ and $\phi^\star$. The final inequality follows from Assumption~\ref{asmp: smooth dynamics}. 
    Combining these results concludes the proof. 
\end{proof}

We now proceed to prove \Cref{thm: doed closeness}. 

\begin{proof}
    The proof follows by modifying the proof of Theorem 3 in \citet{wagenmaker2023optimal}. In place of the regret minimization algorithm used by \citet{wagenmaker2023optimal} to estimate the solution to 
    \begin{align*}
        \min_{\pi \in \Pi_{\exp}} \E_{\pi, \phi^\star}\brac{\sum_{t=1}^T c^m (X_t,U_t)},
    \end{align*}
    we use the policy synthesized directly via optimism over the parameter estimate set $\calB$. Let $\phi_m$ be the parameter value under which the optimistic policy was synthesized and let $\pi^m$ be the optimistic policy.  
    By our assumption that $\phi^\star \in \calB$, the optimistic policy synthesis provides that
    \begin{align*}
          &\E_{\pi^m, \phi^\star}\brac{\sum_{t=1}^T c^m (X_t,U_t)} - \min_{\pi \in \Pi_{\exp}} \E_{\pi, \phi^\star}\brac{\sum_{t=1}^T c^m (X_t,U_t)}\leq \E_{\pi^m, \phi^\star}\brac{\sum_{t=1}^T c^m (X_t,U_t)} -  \E_{\pi^m, \phi_m}\brac{\sum_{t=1}^T c^m (X_t,U_t)}.
    \end{align*}
    By \Cref{lem: self-bounding}, we have that
    \begin{align*}
        \E_{\pi^m, \phi^\star}\brac{\sum_{t=1}^T c^m (X_t,U_t)} -  \E_{\pi^m, \phi_m}\brac{\sum_{t=1}^T c^m (X_t,U_t)} \leq  \frac{T^2 L_f}{\sigma_w} \norm{\phi^\star - \phi^m}. 
    \end{align*}
    By the fact that $D(\calB)$ is the diameter of $\calB$, it follows that the above quantity is bounded as
    \begin{align*}
        \E_{\pi^m, \phi^\star}\brac{\sum_{t=1}^T c^m (X_t,U_t)} -  \E_{\pi^m, \phi_m}\brac{\sum_{t=1}^T c^m (X_t,U_t)} \leq  \frac{T^2 L_f}{\sigma_w} D(\calB). 
    \end{align*}
    
    Substituting this bound in place of the bound form the regret minimization step in the proof of Theorem 3 of \citet{wagenmaker2023optimal}, and carrying out the remaining steps from the proof yields that with probability at least $1-\delta$,
    \begin{align*}
        \Phi(\Delta_{\tilde K}) - \argmin_{\pi \in \Pi_{\exp}} \Phi(\Sigma^{\pi}) \leq \frac{2\beta T^2 L_f^4 \log(\tilde K+1)}{\tilde K+1} + B_{\Phi} \paren{\frac{T^2 L_f D(\calB)}{\sigma_w}  + \sqrt{\frac{8 \log(2 \tilde K/\delta)}{\tilde N}}}.
    \end{align*}
\end{proof}

We now consider the correctness of $\texttt{DOED}_+$ as it is invoked in \Cref{line: doed call} by verifying that the conditions to apply the above result are met. 
\begin{lemma}[Modified from Corollary 1 of \citet{wagenmaker2023optimal}]
    \label{lem: regularized doed objective} Let Assumption~\ref{asmp: smooth dynamics} hold.
    Suppose that $\phi^\star \in \calB$. Let $D(\calB) = \sup_{\phi_1, \phi_2 \in \calB^-} \norm{\phi_1 - \phi_2}$. Assume $\calH \succ 0$, and define the objective $\Phi(\Lambda) \gets \trace(\calH(\Lambda + \lambda I)^{-1})$ for some $\lambda > 0$. Let $B_{\Phi} = T L_f^2 \norm{\calH}_{\op}/\lambda^2$. 
    Then with probability at least $1-\delta$, the data collected at the final round of DOED satisfies
    \begin{align*}
        &\Phi\paren{\frac{1}{(\tilde K+1) \tilde N} \sum_{t,n=1}^{T,((\tilde K+1) \times \tilde N)} D f(X_t^n, U_t^n; \hat \phi)^\top D f(X_t^n, U_t^n; \hat \phi) }- \min_{\pi \in \Pi_{\exp}} \Phi\paren{\E_{\pi, \phi^\star}\brac{ \sum_{t=1}^{T} D f(X_t^1, U_t^1; \hat \phi)^\top D f(X_t^1, U_t^1; \hat \phi)}} \\
        &\leq \frac{2 T^4 L_f^8 \norm{\calH}_{\op}  \log(\tilde N+1)}{\lambda^3 (\tilde N+1)} + \frac{T L_f^2 \norm{\calH}_{\op}}{\lambda^2} \paren{\frac{T^2 L_f D(\calB)}{\sigma_w}  + \sqrt{\frac{8 \log\frac{2\tilde N}{\delta}}{\tilde K}}}.  
    \end{align*}
\end{lemma}
\begin{proof}
    The result follows from \Cref{thm: doed closeness}. The smoothness parameters of Assumpton~\ref{asmp: doed regularity} under the chosen objective are shown in Corollary 1 of \citet{wagenmaker2023optimal} to be bounded as 
    $B_{\Phi} \leq \frac{T L_f^2 \norm{\calH}_{\op}}{\lambda^2}$ and $ \kappa \leq \frac{2 T^2 L_f^4 \norm{\calH}_{\op}}{\lambda^3}$. 
\end{proof}

\begin{lemma}
    \label{lem: good policy for estimate}
    Suppose Assumptions~\ref{asmp: smooth dynamics} and \ref{asmp: good policy} hold. Additionally suppose that $\norm{\hat \phi - \phi^\star}\leq \frac{\lambda_{\min}^\star}{4 T L_f^2}$. Then there exists an exploration policy $\pi \in \Pi_{\exp}$ such that
    \begin{align*}
        \E_{\pi,\phi^\star}\brac{\sum_{t=1}^T Df(X_t, U_t,\hat \phi)^\top D f(X_t, U_t, \hat\phi)} \geq \frac{\lambda_{\min}^\star}{2}.
    \end{align*}
\end{lemma}
\begin{proof}
    The result follows by observing that there exists a policy such that
    \begin{align*}
        \E_{\pi,\phi^\star}\brac{\sum_{t=1}^T Df(X_t, U_t, \phi^\star)^\top D f(X_t, U_t, \phi^\star)} \geq \lambda_{\min}^\star.
    \end{align*}
    by Assumption~\ref{asmp: good policy}. Then 
    \begin{align*}
        &\E_{\pi,\phi^\star}\brac{\sum_{t=1}^T Df(X_t, U_t,\hat \phi)^\top D f(X_t, U_t, \hat\phi)} - \E_{\pi,\phi^\star}\brac{\sum_{t=1}^T Df(X_t, U_t,\hat \phi)^\top D f(X_t, U_t, \hat\phi)} \\&=  \E_{\pi,\phi^\star}\brac{\sum_{t=1}^T \paren{Df(X_t, U_t,\hat \phi)^\top D f(X_t, U_t, \hat\phi) - Df(X_t, U_t, \phi^\star)^\top D f(X_t, U_t, \phi^\star)} }.
    \end{align*}
    By a first order Taylor expansion of $Df(X_t, U_t,\hat \phi)^\top D f(X_t, U_t, \hat\phi)$ about $\phi^\star$, and using the boundedness conditions of Assumption~\ref{asmp: smooth dynamics}, we can bound 
    \begin{align*}
        \norm{\E_{\pi,\phi^\star}\brac{\sum_{t=1}^T \paren{Df(X_t, U_t,\hat \phi)^\top D f(X_t, U_t, \hat\phi) - Df(X_t, U_t, \phi^\star)^\top D f(X_t, U_t, \phi^\star)} } }_{\op}\leq 2T L_f^2 \norm{\hat \phi - \phi^\star} \leq 
        \frac{\lambda_{\min}^\star}{2}.  
    \end{align*}
\end{proof}

\begin{lemma}
    \label{lem: doed PD data}
    Assume that Assumptions~\ref{asmp: smooth dynamics} and \ref{asmp: good policy} hold. Additionally, suppose that $\phi^\star \in \calB$. Let $D(\calB) = \sup_{\phi_1, \phi_2 \in \calB} \norm{\phi_1 - \phi_2}$. Assume $\calH \succ 0$, and define the objective $\Phi(\Lambda) \gets \trace(\calH(\Lambda + \lambda I)^{-1})$. Let $B_{\Phi} = T L_f^2 \norm{\calH}_{\op}/\lambda^2$. Let $\delta \in (0, \frac{1}{2}]$. Suppose $\lambda \leq 
    \frac{\lambda_{\min}(H)\lambda_{\min}^\star}{8\norm{\calH}_{\op} d_{\phi}}$, $D(\calB) \leq \frac{R}{N^{\alpha}}$ and 
    \begin{align*}
        N \geq \max \curly{\left\lceil \frac{4 \lambda_{\min}^\star T^4 L_f^8 \log(N+1)}{\lambda^3 d_{\phi}} \right\rceil^3, \left\lceil \frac{8 \lambda_{\min}^\star T L_f^2  \sqrt{2 \log(2N/\delta)}}{\lambda^2 d_{\phi}} \right\rceil^3, \paren{\frac{4 T^3 L_f^3 R \lambda_{\min}^\star}{\lambda^2 \sigma_w d_{\phi}}}^{1/\alpha}}
        %\paren{\paren{\frac{2 T^4 L_f^8 \norm{\calH}_{\op}  \log(\tilde N+1)}{\lambda^3} + \frac{T L_f^2 \norm{\calH}_{\op}}{\lambda^2} \paren{\frac{T^2 L_f R}{\sigma_w}  + \sqrt{8 \log\frac{2 \tilde N}{\delta}}}}\frac{2 d_{\phi}}{{\lambda_{\min}^\star}}\norm{\calH}_{\op} }^\frac{1}{\alpha}.
    \end{align*}
    Then with probability at least $1-\delta$, the data collected at the final round of $\texttt{DOED}_+$ satisfy
    \begin{equation}
    \label{eq: doed subopt}
    \begin{aligned}
        &\Phi\paren{\frac{1}{\tilde N (\tilde K+1)} \sum_{t,n=1}^{T,(\tilde N \times (\tilde K+1))} D f(X_t^n, U_t^n; \hat \phi)^\top D f(X_t^n, U_t^n; \hat \phi) }- \min_{\pi \in \Pi_{\exp}} \Phi\paren{\E_{\pi, \phi^\star}\brac{ \sum_{t=1}^{T} D f(X_t^n, U_t^n; \hat \phi)^\top D f(X_t^n, U_t^n; \hat \phi)}} \\
        &\leq \frac{2 T^4 L_f^8 \norm{\calH}_{\op}  \log(\tilde K+1)}{\lambda^3 (\tilde K+1)} + \frac{T L_f^2 \norm{\calH}_{\op}}{\lambda^2} \paren{\frac{T^2 L_f D(\calB)}{\sigma_w}  + \sqrt{\frac{8 \log\frac{2 \tilde K}{\delta}}{\tilde N}}}
    \end{aligned}
    \end{equation}
    and 
    \begin{align*}
        \lambda_{\min}\paren{\frac{1}{\tilde N (\tilde K+1)} \sum_{t,n=1}^{T,
    ((\tilde K+1)\times \tilde N)} D f(X_t^n, U_t^n; \hat \phi)^\top D f(X_t^n, U_t^n; \hat \phi)} \geq \frac{\lambda_{\min}(\calH) \lambda_{\min}^\star}{4 \norm{\calH}_{\op} d_{\phi}}.
    \end{align*}
\end{lemma}
\begin{proof}
    By \Cref{lem: regularized doed objective}, we have that with probability at leat $1-\delta$, 
        \begin{align*}
        &\Phi\paren{\frac{1}{\tilde N(\tilde K+1)} \sum_{t,n=1}^{T,(\tilde N \times (\tilde K+1))} D f(X_t^n, U_t^n; \hat \phi)^\top D f(X_t^n, U_t^n; \hat \phi) }- \min_{\pi \in \Pi_{\exp}} \Phi\paren{\E_{\pi, \phi^\star}\brac{ \sum_{t=1}^{T} D f(X_t^1, U_t^1; \hat \phi)^\top D f(X_t^1, U_t^1; \hat \phi)}} \\
        &\leq \frac{2 T^4 L_f^8 \norm{\calH}_{\op}  \log(\tilde K+1)}{\lambda^3 (\tilde K+1)} + \frac{T L_f^2 \norm{\calH}_{\op}}{\lambda^2} \paren{\frac{T^2 L_f D(\calB)}{\sigma_w}  + \sqrt{\frac{8 \log\frac{2 \tilde K}{\delta}}{\tilde N}}} \\ 
        & \leq \frac{2 T^4 L_f^8 \norm{\calH}_{\op}  \log(N+1)}{\lambda^3 (\lfloor N^{1/3} \rfloor+1)} + \frac{T L_f^2 \norm{\calH}_{\op}}{\lambda^2} \paren{\frac{T^2 L_f R}{ N^{\alpha} \sigma_w}  + \sqrt{\frac{8 \log\frac{2 N}{\delta}}{\lfloor N^{2/3} \rfloor}}} \\
        &\leq \frac{ d_{\phi}}{\lambda_{\min}^\star} \norm{\calH}_{\op},
    \end{align*}
    where the final inequality follows from the lower bound on $N$.  By Assumption~\ref{asmp: good policy} paired with \Cref{lem: good policy for estimate}, we have that
    \begin{align*}
        &\min_{\pi \in \Pi_{\exp}} \Phi\paren{\E_{\pi, \phi^\star}\brac{ \sum_{t=1}^{T} D f(X_t^1, U_t^1; \hat \phi)^\top D f(X_t^1, U_t^1; \hat \phi)}}\\&= \trace\paren{\calH \paren{\E_{\pi, \phi^\star}\brac{ \sum_{t=1}^{T} D f(X_t^n, U_t^n; \hat \phi)^\top D f(X_t^1, U_t^1; \hat \phi)} + \lambda I}^{-1} } \leq  \frac{d_{\phi}}{\lambda_{\min}^\star}\norm{\calH}_{\op}. 
    \end{align*}
    We may lower bound 
    \begin{align*}
        \Phi\paren{\frac{1}{\tilde N (\tilde K+1)} \sum_{t,n=1}^{T,(\tilde N \times (\tilde K+1))} D f(X_t^n, U_t^n; \hat \phi)^\top D f(X_t^n, U_t^n; \hat \phi) } \\\geq \frac{\lambda_{\min}\paren{\calH} }{\lambda_{\min}\paren{\frac{1}{\tilde N \tilde K} \sum_{t,n=1}^{T,(\tilde N \times \tilde K)} D f(X_t^n, U_t^n; \hat \phi)^\top D f(X_t^n, U_t^n; \hat \phi)} + \lambda}.
    \end{align*}
    We conclude by combining these inequalities, and using the assumption that $\lambda \leq \frac{\lambda_{\min}(\calH) \lambda_{\min}^\star}{4\norm{\calH}_{\op} d_{\phi }}$.
\end{proof}

\begin{lemma}
    \label{lem: cov and H pert}
    Consider a policy $\pi \in \Pi_{\exp}$. Suppose $\norm{\hat \phi - \phi^\star} \leq \min\curly{\frac{\tilde \lambda}{4 T L_f^2},1}$ for some $\tilde \lambda > 0$. Define
    \begin{align*}
       \Sigma^{\pi}_{\hat\phi} = \E_{\pi, \phi^\star}\brac{ \sum_{t=1}^{T} D f(X_t^n, U_t^n; \hat \phi)^\top D f(X_t^n, U_t^n; \hat \phi)},
    \end{align*}
    and suppose that $\Sigma^{\pi}_{\hat\phi} \succeq \tilde \lambda I$. 
    Then $\Sigma^\pi \succeq \frac{\tilde\lambda}{2} I$, and
    \begin{enumerate}
        \item $\trace\paren{\calH(\phi^\star) \paren{\Sigma^{\pi}}^{-1}} \leq \trace\paren{\calH(\hat\phi) \paren{\Sigma^{\pi}}^{-1}_{\hat\phi}} + \mathsf{poly}\paren{L_{\pi^\star}, L_f, L_{\theta}, L_{\cost}, \sigma_w^{-1},   T, \dx, d_{\phi}, \norm{\calH(\phi^\star)}, \frac{1}{\tilde\lambda}} \norm{\hat \phi - \phi^\star}$
        \item $\trace\paren{\calH(\hat\phi) \paren{\Sigma^{\pi}_{\hat\phi}}^{-1}} \leq\trace\paren{\calH(\phi^\star) \paren{\Sigma^{\pi}}^{-1}} + \mathsf{poly}\paren{L_{\pi^\star}, L_f, L_{\theta}, L_{\cost}, \sigma_w^{-1},  T, \dx, d_{\phi}, \norm{\calH(\phi^\star)}, \frac{1}{\tilde\lambda}} \norm{\hat \phi - \phi^\star}$
    \end{enumerate}
\end{lemma}
\begin{proof}\,\\
To begin, we observe that by a first order Taylor expansion of $D f(x,u; \phi^\star)$ about $\hat\phi$, we have that 
\begin{align*}
    \Sigma^\pi &\succeq \E_{\pi, \phi^\star}\brac{ \sum_{t=1}^{T} D f(X_t^n, U_t^n; \hat\phi)^\top D f(X_t^n, U_t^n; \hat\phi)} + G,
\end{align*}
where $\norm{G} \leq 2 T L_f^2 \norm{\hat\phi-\phi^\star}$ by the boundedness assumptions on the derivatives of $f$ from Assumption~\ref{asmp: smooth dynamics}. By the assumption that $\norm{\hat\phi-\phi^\star}\leq\frac{\tilde\lambda}{4 TL_f^2}$, it holds that $\norm{G} \leq \frac{\tilde\lambda}{2}$. Then it follows that $\lambda_{\min}(\Sigma^\pi) \geq \lambda_{\min}(\Sigma^\pi_{\hat\phi}) - \norm{G} \geq \frac{\tilde \lambda}{2}$. 

\sloppy We proceed to bound $\norm{\paren{\Sigma^\pi}^{-1} - \paren{\hat \Sigma^\pi}^{-1}}$. We immediately have that $\norm{\paren{\Sigma^\pi}^{-1} - \paren{\hat \Sigma^\pi}^{-1}} \leq \frac{1}{\lambda_{\min}\paren{\Sigma^\pi} \lambda_{\min}\paren{\Sigma^\pi_{\hat\phi}}} \norm{\Sigma^\pi_{\hat\phi} - \Sigma^\pi} \leq \frac{2}{\tilde \lambda^2} \norm{\Sigma^\pi_{\hat\phi} - \Sigma^\pi}$. By Taylor expanding $Df(x,u; \hat\phi)$ about $\phi^\star$, we have from the boundedness assumptions of Assumption~\ref{asmp: smooth dynamics} that $\norm{\Sigma^\pi_{\hat\phi} - \Sigma^\pi} \leq 2T L_f^2 \norm{\hat\phi-\phi^\star} + TL_f \norm{\hat\phi-\phi^\star}^2 \leq 3 T L_f^2 \norm{\hat\phi-\phi^\star}$.  Furthermore, by \Cref{lem: model task hessian error},  $\norm{\calH(\hat\phi) - \calH(\phi^\star)}\leq \mathsf{poly}\paren{L_{\pi^\star}, L_f, L_{\theta}, L_{\cost}, \sigma_w^{-1}, T, \dx} \norm{\phi - \phi^\star}. $ 

To conclude, we bound 
\begin{align*}
    \abs{\trace\paren{\calH(\phi^\star) \paren{\Sigma^{\pi}}^{-1}} - \trace\paren{\calH(\phi^\star) \paren{\Sigma^{\pi}_{\hat\phi}}^{-1}}} &\leq \norm{\calH(\phi^\star)} d_{\phi} \norm{\paren{\Sigma^\pi}^{-1} - \paren{\hat \Sigma^\pi}^{-1}}\leq \norm{\calH(\phi^\star)} d_{\phi} \frac{6 T L_f^2 \norm{\hat\phi-\phi^\star}}{\tilde\lambda^2},
\end{align*}
and
\begin{align*}
    \abs{\trace\paren{\calH(\phi^\star) \paren{\Sigma^{\pi}_{\hat\phi}}^{-1}}  - \trace\paren{\calH(\hat\phi) \paren{\Sigma^{\pi}_{\hat\phi}}^{-1}}} &\leq \frac{d_{\phi}}{\tilde\lambda} \norm{\calH(\hat\phi)-\calH(\phi^\star)} \\&\leq \frac{d_{\phi}}{\tilde\lambda}  \mathsf{poly}\paren{L_{\pi^\star}, L_f, L_{\theta}, L_{\cost}, \sigma_w^{-1}, T, \dx} \norm{\phi - \phi^\star}.
\end{align*}
Combining these inequalities with the triangle inequality provides the desired result. 
\end{proof}
